# Supplementary material for: Modeling and Control of an Omnidirectional Micro Aerial Vehicle Equipped with a Soft Robotic Arm
Source: arXiv:2111.03111 source file (2021-11-04)
Supplement: Supplementary file 1 [file 08_appendixes.tex]

\section*{Appendix A: Input Field}
Continuous soft robots actuation systems are of the most disparate kinds, ranging from tendon driven \cite{renda20123d}, to dielectric elastomer \cite{carpi2007folded}. A complete treatise of the modeling of such systems is beyond the scope of the present paper. We refer the interested reader to \cite{rus2015design} for further details. 

We consider here to have an internal wrench independently applied at the two ends of a CC segment. In this case the mapping between the control input and the augmented system joint torques can be expressed as
%
% \begin{equation}
% 	\tau_{\xi} = \sum_{1}^{n} (J_{\xi,\mathrm{a}}^i(\xi) - J_{\xi,\mathrm{a}}^{i-1}(\xi)) \, \tau_i
% \end{equation}
\begin{equation} \label{eq:input}
	\tau_{\xi} = A_{\xi}(\xi)\tau_{\mathrm{a}}
\end{equation}
with
\begin{equation}
\small
A_{\xi}(\xi) = 
	\begin{bmatrix}
    	&\cdots &\vline  &J_{\xi,i}^T(\xi) - J_{\xi,i-1}^T(\xi) \, T_{i}^{i-1}(\xi) &\vline &\cdots &
    \end{bmatrix} \; ,
\end{equation}
where $J_{\xi,i}(\xi)$ is the Jacobian mapping $\dot{\xi}$ into the linear and angular velocities of $S_i$, and  $T_{i}^{i-1}(\xi)$ is the inverse of the homogeneous transformation in \eqref{eq:T}. Combining \eqref{eq:js_m_def} and \eqref{eq:input} yields to 
\begin{equation} \label{eq:input}
	\tau = A(q)\tau_{\mathrm{a}}
\end{equation}
with
\begin{equation}
	A(q) = J_{\mathrm{m}}^T(q) \; A_{\xi}(m(q)).
\end{equation}
Lets consider now a planar PCC soft robot, actuated with internal torques applied at the ends of each segment, as in Fig. \ref{fig:segment_elastic}. This case is of particular interest since it models a xxx actuation \cite{marchese}.
\begin{figure}
	\centering
    \includegraphics[width = 0.7\columnwidth]{dwg/segment_elastic}
    \caption{A segment with constant curvature. An internal torque $\tau_i$ is applied at both ends. The radius of the segment section is $\Delta$. A spring and a damper are connected through the arc at distance $\delta$ from the segment axis. \label{fig:segment_elastic}}
\end{figure}
Interestingly in this case $A(q)$ is the identity matrix. This is coherent with the discussed property of the PCC model, to exactly describe the kinematic in the case of constant torque applied at the end of the segment.

\section*{Appendix B: Impedance}

The effect of elastic and viscous dissipative fields can be easily described by introducing the first one in $G_{\xi}$, and the second one in $C_{\xi}\dot{\xi}$, in \eqref{eq:xidyn}. However, it is more convenient to evaluate the impedance directly in the PCC soft robot space $q$, $\dot{q}$. We will consider here the planar case described in Fig. \ref{fig:segment_elastic}. We model the link elasticity through a continuous distribution of infinitesimal elastic terms, along the whole segment area. From simple geometrical considerations, the length of an infinitesimal spring at distance $\delta$ from the central axis of the segment is 
\begin{equation}
 	L_{\delta,i}(q_i) = (\frac{L_i}{q_i} - \delta) \, q_i \, ,
\end{equation}
where $L_i$ is the length of the central axis of the segment (constant for every $q_i$ by construction).
We consider the spring to be linear, with an amount of stored energy equal to 
\begin{equation}
	\begin{split}
		E_{\delta,i}(q_i) &= \frac{1}{2} \kappa_i (L_{\delta,i}(0) - L_{\delta,i}(q_i))^2 \\
                          &= \frac{1}{2} \kappa_i \delta^2 q_i^2 \, .
	\end{split}
\end{equation}
Thus, the total amount of energy stored in the segment area is 
\begin{equation}
	E_{i}(q_i) = \int_{-\Delta}^{+\Delta} E_{\delta,i}(q_i) \mathrm{d} \delta = \frac{2}{3} \kappa_i \Delta^3 q_i^2.
\end{equation}
The elastic force acting on the i\--th segment can then be evaluated as
\begin{equation}
	\frac{\partial E_{i}(q_i)}{\partial q_i} = \frac{4}{3} \kappa_i \Delta^3 q_i.
\end{equation}
Which is linear in the curvature angle $q_i$. A linear model of spring w.r.t. the local curvature is indeed coherent with the continuous Hooke model \cite{}.

Similarly we introduce a damper in parallel to each infinitesimal spring. We consider a linear friction model, for which the generated force is equal to $\beta \, \dot{L}_{\delta,i}$. By exploiting kineto-static duality and integrating over the surface, we obtain the total dissipative force produced at the i\--th segment
\begin{equation}
	\int_{-\Delta}^{\Delta} \beta_i \left(\frac{\partial L_{\delta,i}}{\partial q_i}\right)^2 \dot{q}_i \; \mathrm{d} \delta = \frac{4}{3} \beta_i \Delta^3 \dot{q}_i \; .
\end{equation}
So in the PCC hypotheses damping and elastic actions can be described by two linear terms, $D \, \dot{q}$ and $K \, q$ respectively, where $D$ and $K$ are two diagonal matrices, with $\frac{4}{3} \kappa_i \Delta^3$ and $\frac{4}{3} \beta_i \Delta^3$ as i\--th diagonal elements.
